# Supplementary material for: Non-uniform carrier density in Cd$_3$As$_2$ evidenced by optical spectroscopy
Source: arXiv:1712.03147 source file (2018-03-11)
Supplement: Supplementary file 1 [file SI.pdf]

# Supplementary Material for "Non-uniform carrier density in $Cd_3As_2$ evidenced by optical spectroscopy"

I. Crassee,[1] E. Martino,[2] C. C. Homes,[3] O. Caha,[4] J. Novák,[4] P. Tückmantel,[5] M. Hakl,[1] A. Nateprov,[6] E. Arushanov,[6] Q. D. Gibson,[7] R. J. Cava,[7] S. M. Koohpayeh,[8] K. E. Arpino,[8,9] T. M. McQueen,[8,9,10] M. Orlita,[1,11] and Ana Akrap[5,*]

[1]*LNCMI, CNRS-UGA-UPS-INSA, 25, avenue des Martyrs, F-38042 Grenoble, France*
[2]*IPHYS, EPFL, CH-1015 Ecublens, Switzerland*
[3]*Condensed Matter Physics and Materials Science Department, Brookhaven National Laboratory, Upton, New York 11973, USA*
[4]*CEITEC and Masaryk University, Faculty of Science, CZ-61137 Brno, Czech Republic*
[5]*DQMP, University of Geneva, CH-1211 Geneva 4, Switzerland*
[6]*Institute of Applied Physics, Academy of Sciences of Moldova, MD-2028 Chisinau, Moldova*
[7]*Department of Chemistry, Princeton University, Princeton, New Jersey 08544, USA*
[8]*Institute for Quantum Matter and Department of Physics and Astronomy, The Johns Hopkins University, Baltimore, Maryland US-21218, USA*
[9]*Department of Chemistry, The Johns Hopkins University, Baltimore, Maryland US-21218, USA*
[10]*Department of Materials Science and Engineering, The Johns Hopkins University, Baltimore, Maryland US-21218, USA*
[11]*Institute of Physics, Charles University in Prague, CZ-12116 Prague, Czech Republic*

(Dated: February 16, 2018)

In the Supplementary Material we show additional data supporting the conclusions of the main text. First, we fits to the reflectivity data to illustrate the extraction of the Drude scattering and its influence on the reflectivity. We continue with the effect of polishing on the high energy optical properties. Then we show the temperature dependent optical spectra for samples A, C and D from the main manuscript (sample B is discussed in the main text). Following this, we show evidence that the carrier concentration reduces over time. Finally, we show results of the high pressure infrared transmission.

## I. EXTRACTING THE DRUDE SCATTERING RATE

In order to extract the Drude plasma frequency $\omega_p$ and scattering rate $1/\tau$, we fit the reflectance data using a standard Drude-Lorentz model for the dielectric function:

$$\tilde{\epsilon}(\omega) = \epsilon_\infty - \frac{\omega_p^2}{\omega^2 + i\omega/\tau} + \sum_k \frac{\Omega_k}{\omega_k^2 - \omega^2 - i\omega\gamma_k},$$

where $\omega_k$, $\gamma_k$, and $\Omega_k$ are the position, width, and strength of the $k$th vibration, respectively.

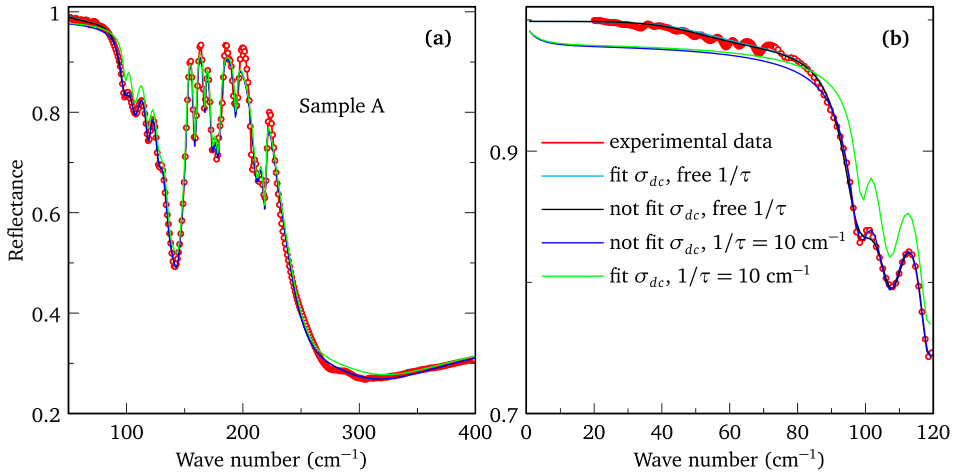


Fig. S1. Experimental reflectance data on sample A, shown together with fits using Drude-Lorentz models.

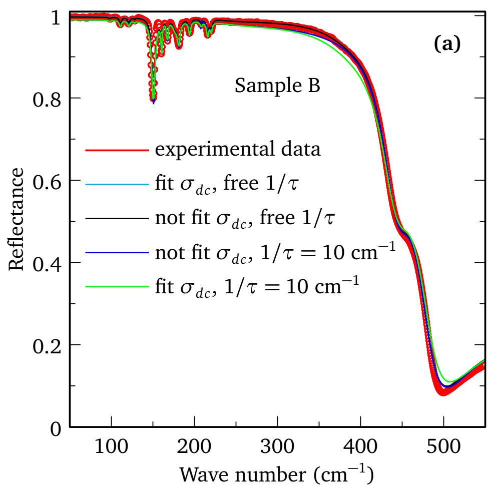


Fig. S2. Experimental reflectance data on sample B, together with fits using Drude-Lorentz models.

Figs. S1 and S2 show several different fits to the data, where the scattering rate $1/\tau$ was either fitted ("free $1/\tau$") or fixed to 10 cm$^{-1}$. Similarly, $\sigma_{dc}$ was either fitted ("fit") or it was disregarded ("not fit"). In the main text, we report results from fitting both $1/\tau$ and $\sigma_{dc}$. While the fitted values of $1/\tau = 0.6$ cm$^{-1}$ for sample A, and $1/\tau = 2$ cm$^{-1}$ for sample B, are extremely small, the estimated confidence limit for both samples is much larger, $\Delta\tau \sim 10$ cm$^{-1}$. This means that the fits shown in Figs. S1 and S2 with $1/\tau \sim 10$ cm$^{-1}$ are still considered acceptable. For a freely fitted $1/\tau$ parameter, including or excluding $\sigma_{dc}$ makes no significant difference. When the parameter $1/\tau$ is taken at the edge of the confidence interval, 10 cm$^{-1}$, the fit becomes significantly less good. In particular, a fit with a higher $1/\tau$ fails to describe the sharp plasma edge observed in sample B, seen around 300 cm$^{-1}$.

## II. POLISHING AND THE HIGH-ENERGY OPTICAL PROPERTIES

In many experiments it is necessary to cut and/or polish the samples of $Cd_3As_2$. However, it is highly likely that this mechanical treatment damages or chemically alters a thin surface layer. To demonstrate this, Fig. S3 shows the real ($\epsilon_1$) and imaginary ($\epsilon_2$) parts of the complex dielectric function for three samples. All three samples originate from the same batch of single crystals.

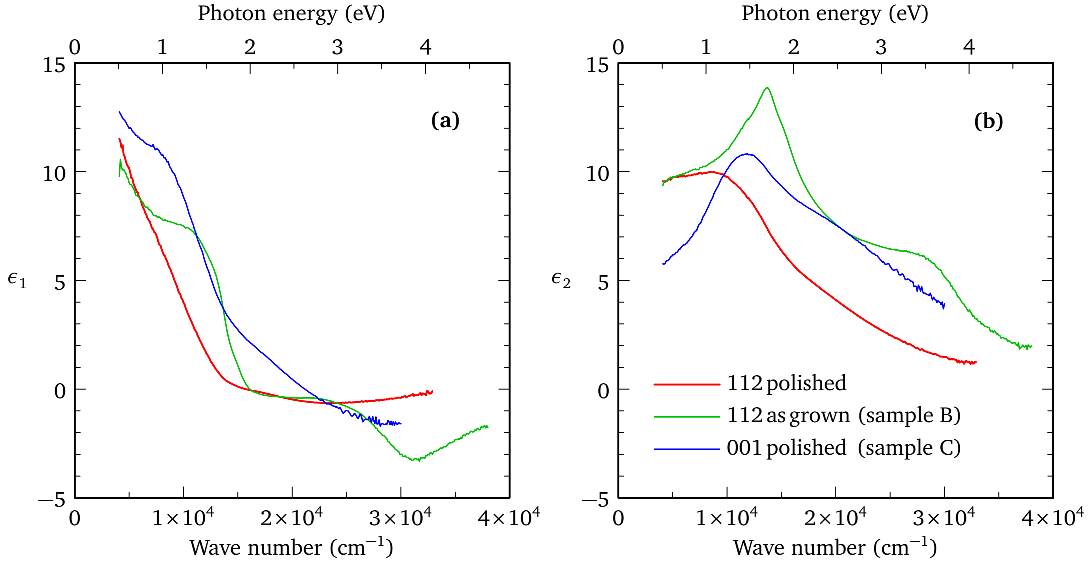


Fig. S3. (a) Real and (b) imaginary parts of the complex dielectric function $\tilde{\epsilon}$, determined by ellipsometry at room temperature on three samples from the same batch.

In the as-grown sample B, there are two strong peaks in $\epsilon_2$ at 1.7 eV and 3.7 eV. In contrast, neither of the polished samples shows the 3.7 eV peak. In both polished samples the 1.7 eV peak is broadened and shifted to lower energies. This indicates a chemical reaction taking place on the surface of the sample after it has been polished, possibly involving a reduced amount of Arsenic as compared to the bulk crystals. The polished samples were polished using diamond paper, and kept in the same conditions as the pristine sample B.

## III. TEMPERATURE DEPENDENCE OF REFLECTANCE AND OPTICAL CONDUCTIVITY

Fig. S4 shows the temperature-dependent optical spectra taken on samples A, C and D. Reflectance and the real part of the optical conductivity, $\sigma_1$, are displayed for various temperatures. Data for the sample B are shown and discussed in Fig. 3 of the main text.

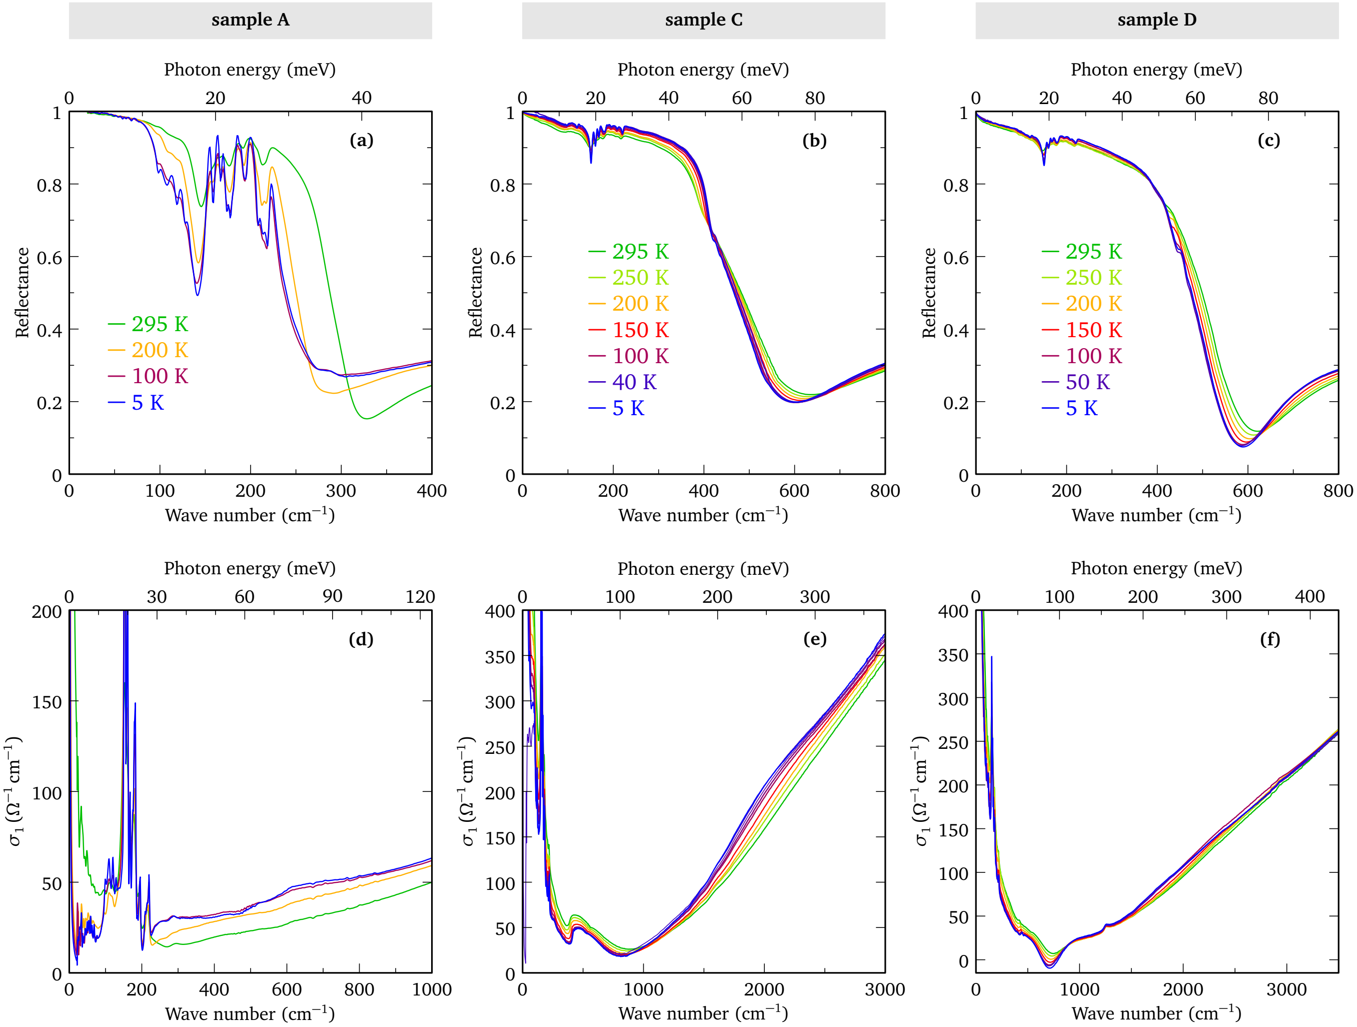


Fig. S4. Optical reflectivity as a function of photon energy shown for different temperatures for (a) sample A, (b) sample C, and (c) sample D. Real part of optical conductivity, $\sigma_1$, shown for different temperatures for (d) sample A, (e) sample C, and (f) sample D.

In all three samples shown, the screened plasma frequency shifts to lower energies as temperature decreases. The decrease in the Drude plasma frequency is most appreciable in sample A, which has the lowest value of chemical potential. The 25% change of the Drude plasma frequency reflects the thermally excited free carriers.
A small step in reflectance develops at low temperature in the vicinity of the screened plasma frequency. As discussed in the main text, we attribute this complex shape of the plasma edge to charge puddles, or a non-uniform carrier concentration on a micrometer scale.

A quasi-linear slope is present in all of the $\sigma_1$ curves. However, a truly linear optical conductivity can only be found in the sample with the lowest carrier concentration (sample A), and also only at low temperatures. As a function of temperature one can discern a clear definition of the Pauli blocking edge, which appears as a kink in $\sigma_1$ at 70 meV in sample A, and above 200 meV in sample C. A similar kink is not obvious in sample D.

## IV. DECREASE OF CHARGE DENSITY AND ANNEALING OF CADMIUM VACANCIES

It has been known that $Cd_3As_2$ samples anneal at room temperature, wherein cadmium atoms progressively order within the tetrahedral voids of the crystal structure.[1] This atomic diffusion happens on a time scale of months or even years. This reduction of carrier concentration over time is reflected in changes of the plasma frequency. The plasma edge shifts significantly to lower energies as a function of time. Fig. S5 shows this on samples B, C and D. This is an effect that we observe in all the measured samples. From the relative change in plasma frequency one can estimate that the carrier density changes by almost 50% in sample B, and by more than 35% in samples C and D.

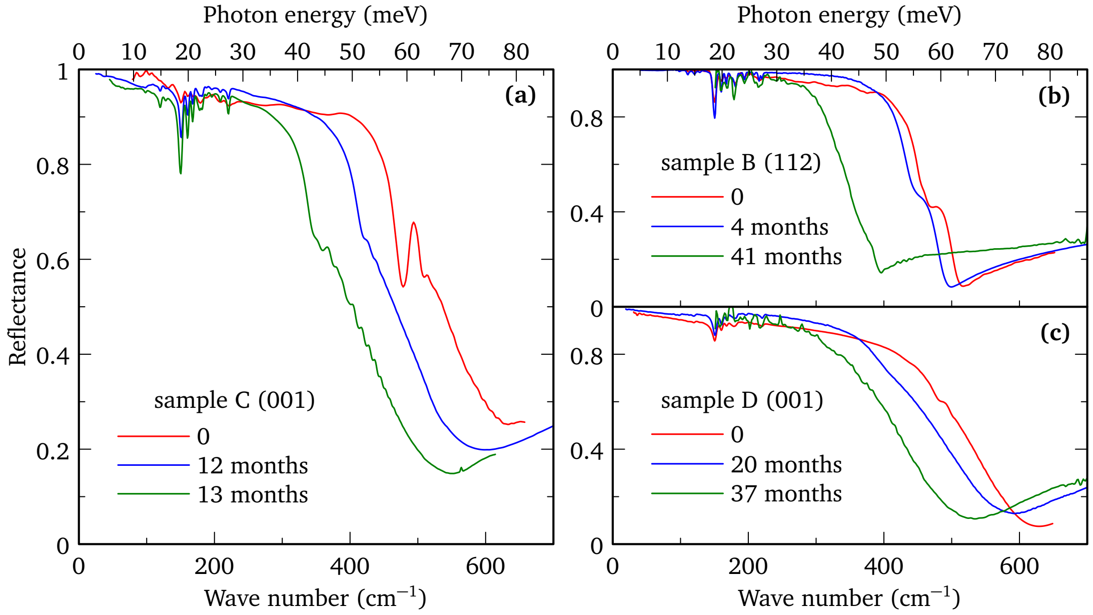


Fig. S5. Reflectance at 5 K is shown as a function of photon energy for samples (a) C, (b) B and (c) D. For each sample the reflectance was measured during three cooling cycles, over several months. The elapsed time is shown with respect to the first measurement. A strong redshift of the screened plasma frequency is observed in each case.

## V. SIMULATION OF CHARGE PUDDLES IN REFLECTIVITY SPECTRA

We can simulate the reflectance in case of a non-homogeneous or anisotropic sample. The measured reflectance will be a weighed average of all the different contributions:

$$R = \sum_i \alpha_i R_i.$$

In the case of charge puddles, $\alpha_i$ corresponds to the portion of the sample which has $i$th carrier density. In the case of anisotropic response, each $i$ represents reflectance with polarization along a projection of the optical axis. For the simulation, we take $\epsilon_\infty = 5$, and Drude plasma frequency ranges from 800 cm$^{-1}$ to 1000 cm$^{-1}$.
Figure S6(a) shows the averaged reflectance around the plasma edge for two equally weighing contributions. This is similar to the reflectance measured in samples with a (112) orientation, as can be observed for example in Fig. S5(b), see the red and blue curves. Figure S6(b) shows the calculation for the case where six different contributions are present. Such a situation corresponds better to the charge puddle scenario. No strong features are present on the plasma edge, but the edge is broadened, similar to Fig. S5(a) and (c).

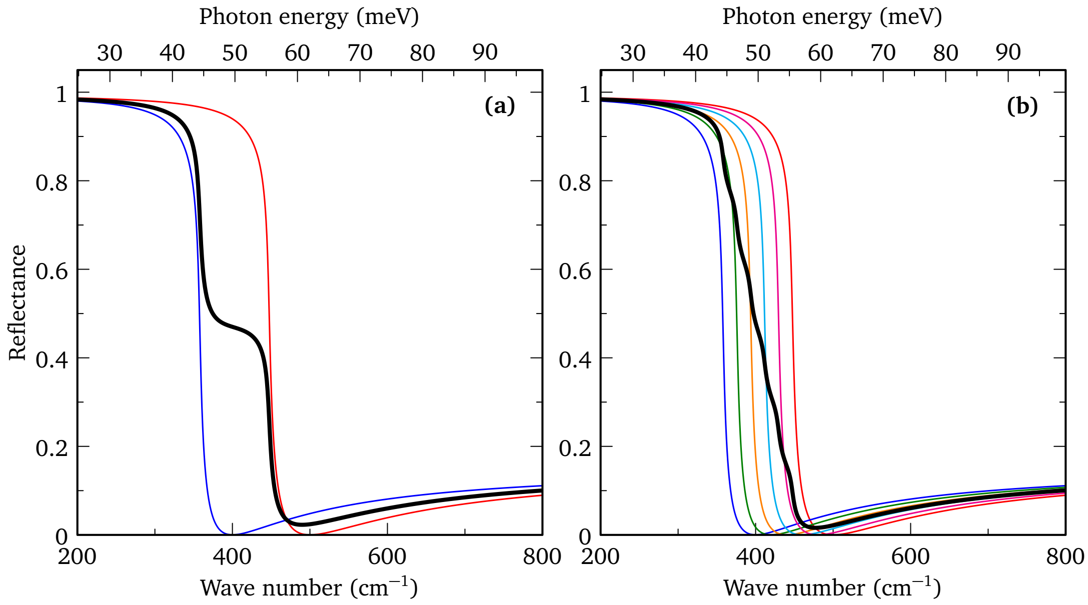


Fig. S6. Simulated reflectance calculated for the case of (a) two contributions and (b) six contributions with different plasma frequencies. In both cases different contributions are given equal weight.

## VI. HIGH PRESSURE INFRARED TRANSMISSION

At high pressure, $p \sim 8.5$ GPa, superconductivity sets in and remains present up to at least 50 GPa,[2] with the critical temperature never exceeding $T_c \sim 4$ K. X-ray measurements show that the semimetallic phase collapses above 3 GPa.

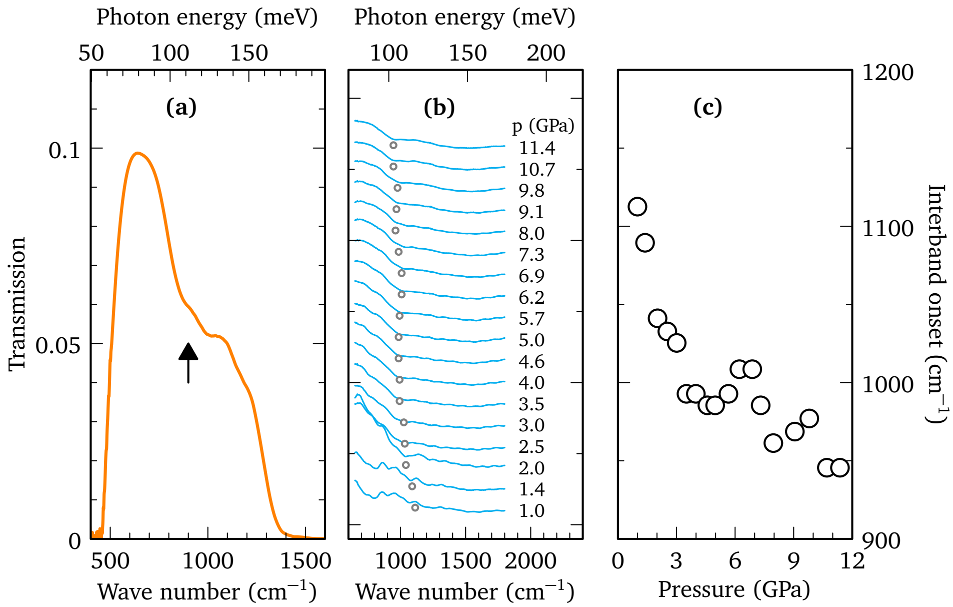


Fig. S7. (a) Transmission at 10 K through the 80 $\mu$m thick sample A′. The arrow points to the drop in transmission, tentatively associated with the onset of the interband absorption. (b) A series of transmission curves (arbitrary units) for different pressures, taken at room temperature in a diamond anvil cell. Open symbols indicate the estimated interband transition onset. (c) Energy of the onset of interband absorption as a function of pressure.

Using a diamond anvil pressure cell and a synchrotron light source, we measured the high pressure infrared transmission up to 11.4 GPa. The spectra were taken at room temperature, with light traversing a several micron thick flake of sample A.

Transmission is linked to absorption, and therefore to $\sigma_1$. Here we only address the normal state as our transmission measurements were limited to room temperature.
Transmission is measurable only when the absorption is small, hence we focus on the low energy properties. High energies, based on reflectivity measurement, are addressed in the Ref. 3. At low energies where the absorption is small, transmission is more sensitive than reflection.
Fig. S7(a) shows the infrared transmission through a piece of sample A' of thickness 80 $\mu$m at 10 K. At low energies transmission is practically zero due to the light absorption by itinerant carriers. Above 170 meV transmission drops to zero within our experimental accuracy, this time due to the interband excitations. Important to our results is an observed change in slope of transmission at 110 meV, which roughly coincides with the onset of interband absorption in $\sigma_1$.
Fig. S7(b) shows a series of spectra, offset by a constant value. The lowest pressure can be taken as ambient pressure. The dominant feature is a change of slope just above 100 meV, similar to the sample outside the cell. We identify the change of slope with the onset of interband transition, or $E_F$ as discussed previously. Above 170 cm$^{-1}$ the infrared transmission has another, albeit weaker inflection point. However, it does not drop to zero, possibly due to a small leak of synchrotron light through the diamond anvil cell. As a function of pressure, transmission drops slightly at frequencies below the change of slope, and increases above this frequency. The position of the step shifts slightly at first to higher energies, then to lower energies.
Fig. S7(c) shows the energy of the step (or change of slope), which we attribute to the onset of interband absorption. The step position monotonically decreases with pressure, without significant changes up to 12 GPa.
A decreasing onset of interband absorption implies that Pauli blocking is decreasing. If the band structure does not change close to the Fermi level, our observation would imply that the Fermi velocity decreases as a function of pressure. In this energy window and at room temperature, we observe no major changes to the band structure.

* ana.akrap@unige.ch

[1] E. K. Arushanov, Progress in Crystal Growth and Characterization **3**, 211 (1981).
[2] L. He, Y. Jia, S. Zhang, X. Hong, C. Jin, and S. Li, Npj Quantum Materials **1**, 16014 EP (2016).
[3] E. Uykur, R. Sankar, D. Schmitz, and C. A. Kuntscher, (2017), arXiv:1708.00725 [cond-mat.mtrl-sci].
